# Supplementary material for: Polarized User and Topic Tracking in Twitter
Source: arXiv:1610.08686 source file (2016-10-27)
Supplement: Supplementary file 1 [file appendix.tex]

%!TEX root = main.tex

\clearpage%\newpage
\appendix

\section{Comments on current work}

\subsection{Tweets and Users classification}

The tweets classification could be done in a more tolerant way,
e.g., according to the majority of hashtags, or a fuzzy classification.

The classification of users could be done on the basis of the user' full stream
and not only on the basis of the classified tweets. Also in this case the classification
might be fuzzy, i.e., assign a probability for each class.

\section{Comments on future work}

\subsection{Expectation Maximization}

\begin{algorithm}
\caption{\label{alg:em-iterative} \myalgo Algorithm}
\begin{algorithmic}[1]
\Require The set of users \users and their tweets \tweets with hashtags \htags,
\Statex \hspace{2.5em} an hashtag $H_c^{0}$ for each class $c \in \topics$
\Ensure Classification of users $U_c$ and hashtags $H_c$
\Procedure{\myalgo}{$H_c^{0}$}
\State $t \gets 0$
\Repeat
\Statex \Comment{Classify users on the basis of the hashtags used}
%\State $\forall u\quad u^{t+1} = \argmax_{c \in \topics}\PR(c | \tweets_u, H^t)$ 
\State $U_c^{t+1} = \PR(c | H_c^{t})$ 

\Statex \Comment{Find better hashtags on the basis of $U_c^{t+1}$}
\State $H_c^{t+1} = \PR(h | U_c^{t+1})$

\State $t \gets t+1$
\Until{ {\em convergence} }
\State \textbf{return} $U_c^{t}$, $H_c^{t}$
\EndProcedure
\end{algorithmic}
\end{algorithm}

The algorithm can be formalized and implemented as an Expectation/Maximization
algo.
